# Supplementary material for: Challenges in Partially-Automated Roadway Feature Mapping Using Mobile Laser Scanning and Vehicle Trajectory Data
Source: arXiv:1902.03346 source file (2019-02-09)
Supplement: Supplementary file 1 [file appendix.tex]

Numerous ITS applications have been identified with the potential to improve mobility, safety, and the environment [24-26]. Connected vehicle technology has been identified as an enabling technology for many of the identified applications. The V2V and V2I connected vehicle im-plementations often require accurate positional information relative to a reference map. The reference map contains road features, such as, lane markings, stop bars, road edges, turn pock-ets and intersection geometry. The goal of this section is to discuss mapping and real-time po-sitioning tradeoffs and to characterize the accuracy requirements of a variety of connected ve-hicle applications. For a common list of connected vehicle applications, we reference the CVRIA (http://www.iteris.com/cvria/). The CVRIA CV application list is based on the results of an extensive connected vehicle research program carried out by the USDOT over the last decade.

he Figure \ref{fig:cvapp} illustrates a connected vehicle maneuvering within a lane near an intersection. Various quantities of interest for the application – forward distance $s_F$, left distance $s_L$, and right distance $s_R$ – are illustrated.  Each of these quantities is computed in real-time at a high rate by differencing the vehicle position $p_V$ with a quantity computed from the map information: $p_L$, $p_F$ or $p_R$. For example, $s_F = p_F - p_V$, each of which is uncertain, with uncertainty indicated in the figure by the size of the concentric circles around the point. Therefore, the uncertainty in the computed quantity is related to the uncertainty in the positions. If we characterize the uncertainty by a standard deviation, then the equation is
\begin{equation}\label{eq:tradeoff}
\sigma_{s_F} = \sqrt{(\sigma_{p_V})^2 + (\sigma_{p_F})^2}
\end{equation}

\begin{figure}
	\begin{center}
		\begin{tabular}{c}
			\includegraphics[height=4cm]{cvapp2.jpg}
		\end{tabular}
	\end{center}
	\caption[example] 
	%>>>> use \label inside caption to get Fig. number with \ref{}
	{ \label{fig:cvapp} 
		CV application variable definitions.}
\end{figure} 

This equation is important as it shows the tradeoff between the accuracy specifications of the map features denoted by $\sigma_{p_F}$ and the implied accuracy requirements for real-time positioning (i.e., navigation) denoted by $\sigma_{p_V}$.
\begin{figure}
	\begin{center}
		\begin{tabular}{c}
			\includegraphics[height=7cm]{accuracy2.jpg}
		\end{tabular}
	\end{center}
	\caption[example] 
	%>>>> use \label inside caption to get Fig. number with \ref{}
	{ \label{fig:cvapp} 
		CV Mapping and positioning }
\end{figure} 
  
Fig. 1.6 illustrates this tradeoff.  Assume that for a given application, the distance to the stop bar $||s_F ||$ must be computed with a standard deviation of less than one meter.  The outermost curve in the figure shows the locus of points that satisfy this specification.  If for example, the map is accurate to 10 cm, then real-time vehicle position estimated to 0.99 meter accuracy is sufficient.  However, if the map is only accurate to 0.9m, then the vehicle position must be estimated in real-time to an accuracy of approximately 40 cm.
